# Supplementary material for: Grid-Aware Islanding and Resynchronisation of AC/DC Microgrids
Source: arXiv:2503.04597 source file (2025-03-06)
Supplement: Supplementary file 1 [file AppendixB.tex]

\section{Interfacing Converter Losses}
\label{appendix:losses}

\textcolor{orange}{
\subsection{Load flow Jacobian}
The interfacing converters' losses are presented in \eqref{eq:losses}. The expression is dependent on the AC and DC currents, which are not in the set of state variables. Therefore, these currents are first reformulated as the AC and DC voltages using the admittance matrix $Y$. The same terminology as in Section \ref{Sec:Model} is used. To reduce the length of the expressions, we assume the IC bus is only connected to one other bus in the AC grid and in the DC grid.
The DC currents are reformulated as:
\begin{flalign}
    & I_{dc} = G_{(k,k)} E_k +  G_{(k,j)} E_j, \nonumber \\
    & I_{dc}^2 = G_{(k,k)}^2 E_k^2 + 2 G_{(k,k)} G_{(k,j)} E_k  E_j + G_{(k,k)}^2 E_j^2.
     \label{eq:losses_2}
\end{flalign}
The AC currents are reformulated as:
\begin{flalign}
    & \overbar{I}_{ac} = \overbar{Y}_{(l,l)} \overbar{E}_l +  \overbar{Y}_{(l,i)} \overbar{E}_l \nonumber \\
    & \overbar{I}_{ac} = \Big( G_{(l,l)} E_l^{\prime} - B_{(l,l)} E_l^{\prime \prime} + G_{(l,i)} E_i^{\prime} - B_{(l,i)} E_i^{\prime \prime}  \Big) + \nonumber \\ 
    & \hspace{22pt} j \Big( B_{(l,l)} E_l^{\prime} + G_{(l,l)} E_l^{\prime \prime} + B_{(l,i)} E_i^{\prime} + G_{(l,i)} E_i^{\prime \prime}\Big) \label{eq:losses_3-} \\
    & \hspace{14pt} = \alpha({  \overbar{E_l}, \overbar{E_i}  }) + j \beta({  \overbar{E_l}, \overbar{E_i}  }), 
     \label{eq:losses_3}
\end{flalign}
Equation \eqref{eq:losses_3-} is simplified by introducing the variables $\alpha$ and $\beta$. 
The AC currents magnitude is reformulated as \eqref{eq:losses_4}. These expressions only depend on the nodal voltages, i.e., the grid states.
\begin{flalign}
    & \lvert \overbar{I}_{ac} \rvert = \sqrt{\alpha({ \scriptstyle \overbar{E_l}, \overbar{E_i}  })^2 + \beta({ \scriptstyle \overbar{E_l}, \overbar{E_i}  })^2} \nonumber \\
    & \lvert \overbar{I}_{ac} \rvert^2 = \alpha({ \scriptstyle \overbar{E_l}, \overbar{E_i}  })^2 + \beta({ \scriptstyle \overbar{E_l}, \overbar{E_i}  })^2 
     \label{eq:losses_4}
\end{flalign}
The partial derivatives of power losses with respect to the AC and DC state variables are given in \eqref{eq:losses_5}. These are substituted in \eqref{eq:VVextra_2} to construct the load flow Jacobian.
\begin{flalign}
    & \frac{\partial P^{loss}_{(l,k)}}{\partial E_i^{\prime}} = \big( V_0 \frac{1}{2 {\scriptstyle \sqrt{\alpha^2 + \beta^2}}} + R_0 \big) \Big( \hspace{12pt} 2 \alpha G_{(l,i)} +  2 \beta B_{(l,i)} \Big)  \nonumber \\
    & \frac{\partial P^{loss}_{(l,k)}}{\partial E_i^{\prime \prime}} = \big( V_0 \frac{1}{2 {\scriptstyle \sqrt{\alpha^2 + \beta^2}}} + R_0 \big) \Big(-2 \alpha B_{(l,i)} +  2 \beta G_{(l,i)} \Big) \nonumber  \\
    & \frac{\partial P^{loss}_{(l,k)}}{\partial E_l^{\prime }} = \big( V_0 \frac{1}{2 {\scriptstyle \sqrt{\alpha^2 + \beta^2}}} + R_0 \big) \Big( \hspace{12pt} 2 \alpha G_{(l,l)} +  2 \beta B_{(l,l)} \Big) \nonumber  \\
    & \frac{\partial P^{loss}_{(l,k)}}{\partial E_l^{\prime \prime }} =  \big( V_0 \frac{1}{2 {\scriptstyle \sqrt{\alpha^2 + \beta^2}}} + R_0 \big) \Big(-2 \alpha B_{(l,l)} +  2 \beta G_{(l,l)} \Big) \nonumber  \\
    & \frac{\partial P^{loss}_{(l,k)}}{\partial E_k} = v G_{(k,k)} + 2 w G_{(k,k)}^2 E_k + 2 w G_{(k,k)} G_{(k,j)} E_j \nonumber \\
    & \frac{\partial P^{loss}_{(l,k)}}{\partial E_j} = v G_{(k,j)} + 2 w G_{(k,j)}^2 E_j + 2 w G_{(k,k)} G_{(k,j)} E_k \nonumber \\
     \label{eq:losses_5}
\end{flalign}
for brevity the dependence of $\alpha$ and $\beta$ on $(\overbar{E_l}, \overbar{E_i} )$ is not explicitly written.
}

\textcolor{orange}{
\subsection{Sensitivity coefficient model}
The SC model in equation \eqref{eq:sc_4} depends on the IC power losses: $\frac{\partial P^{loss}_{(l,k)} }{\partial x}$. This term is computed by taking the partial derivative of \eqref{eq:losses} (or \eqref{eq:losses_6}) to $x$.
\begin{flalign}
    & P^{loss}_{(l,k)} = V_0 \sqrt{\alpha({ \scriptstyle \overbar{E_l}, \overbar{E_i}  })^2 + \beta({ \scriptstyle \overbar{E_l}, \overbar{E_i}  })^2}  \nonumber \\  
    &+ R_0 \Big(\alpha({ \scriptstyle \overbar{E_l}, \overbar{E_i}  })^2 + \beta({ \scriptstyle \overbar{E_l}, \overbar{E_i}  })^2 \Big) \nonumber \\
    &+ u + v (G_{(k,k)} E_k +  G_{(k,j)} E_j ) \nonumber \\
    &+ w (G_{(k,k)}^2 E_k^2 + 2 G_{(k,k)} G_{(k,j)} E_k  E_j + G_{(k,k)}^2 E_j^2). \label{eq:losses_6}
\end{flalign}
\begin{flalign}
    \frac{\partial P^{loss}_{(l,k)} }{\partial x} & =
    \big( V_0 \frac{1}{2 {\scriptstyle \sqrt{\alpha^2 + \beta^2}}} + R_0 \big) \Big( \ 2 \alpha G_{(l,i)} +  2 \beta B_{(l,i)} \Big)   \frac{\partial E_i^{\prime}}{\partial x} \nonumber \\
    & + \big( V_0 \frac{1}{2 {\scriptstyle \sqrt{\alpha^2 + \beta^2}}} + R_0 \big) \Big(\text{-}2 \alpha B_{(l,i)} +  2 \beta G_{(l,i)} \Big) \frac{\partial E_i^{\prime \prime}}{\partial x} \nonumber  \\
    &+ \big( V_0 \frac{1}{2 {\scriptstyle \sqrt{\alpha^2 + \beta^2}}} + R_0 \big) \Big( \ 2 \alpha G_{(l,l)} +  2 \beta B_{(l,l)} \Big) \frac{\partial E_l^{\prime}}{\partial x} \nonumber  \\
    &+\big( V_0 \frac{1}{2 {\scriptstyle \sqrt{\alpha^2 + \beta^2}}} + R_0 \big) \Big(\text{-}2 \alpha B_{(l,l)} +  2 \beta G_{(l,l)} \Big) \frac{\partial E_l^{\prime \prime}}{\partial x} \nonumber  \\
    & + \big( v G_{(k,j)} + 2 w G_{(k,j)}^2 E_j + 2 w G_{(k,k)} G_{(k,j)} E_k \big) \frac{\partial E_j}{\partial x} \nonumber  \\
    & + \big( v G_{(k,k)} + 2 w G_{(k,k)}^2 E_k + 2 w G_{(k,k)} G_{(k,j)} E_j \big) \frac{\partial E_k}{\partial x} 
\end{flalign}
This expression is a linear combination of the voltage partial derivatives and a constant term that is only dependent on the grid's state, admittance matrix and loss parameters. Therefore, it is substituted in \eqref{eq:sc_4} to express the losses in function of the nodal AC and DC voltages. }
