# Supplementary material for: Grid-Aware Islanding and Resynchronisation of AC/DC Microgrids
Source: arXiv:2503.04597 source file (2025-03-06)
Supplement: Supplementary file 2 [file AppendixA.tex]

\section{Construction of the Load Flow Jacobian}
\label{appendix:Jac}

\textcolor{orange}{The elements of the load flow Jacobian matrix for the grid-forming converter are derived by taking the partial derivative of expression \eqref{eq:VVextra_1} (Section \ref{Sec:Model}). 
\footnotesize
\begin{flalign}
    & \frac{\partial E_l^{\ast \prime}}{\partial E_i^{\prime}} \! = \! \frac{\text{-} G_{(l.i)}}{2a} + \frac{1}{2a} \frac{1}{2 \sqrt{b^2 - 4 a c} } \Big( 2 b G_{(l.i)} \! - \! 4 a \big(  B_{(l,i)} E_l^{\prime \prime}  \! + \! \frac{\partial P^{loss}_{(l,k)} }{\partial E_i^{\prime} } \big)  \Big) \nonumber \\
    & \frac{\partial E_l^{\ast \prime}}{\partial E_i^{\prime \prime}} \! = \! \frac{ B_{(l.i)}}{2a} + \frac{1}{2a} \frac{1}{2\sqrt{b^2 - 4 a c} } \Big( \text{-} 2 b B_{(l.i)} \! - \! 4 a \big(  G_{(l,i)} E_l^{\prime \prime} \! + \! \frac{\partial P^{loss}_{(l,k)} }{\partial E_i^{\prime \prime} } \big)  \Big) \nonumber  \\
    & \frac{\partial E_l^{\ast \prime}}{\partial E_l^{\ast \prime }} \! = \!  1 \nonumber  \\
    & \frac{\partial E_l^{\ast \prime}}{\partial E_l^{\prime \prime }} \! = \! \frac{1}{2a} \frac{1}{2\sqrt{b^2 - 4 a c} } \Big( \text{-} 4 a \big( 2 G_{(l,l)}  {E_l^{\prime \prime}} \! + \! G_{(l,i)} E_i^{\prime \prime} \! + \! B_{(l,i)} E_i^{\prime} \! + \! \frac{\partial P^{loss}_{(l,k)} }{\partial E_l^{\prime \prime} } \big) \Big) \nonumber  \\
    & \frac{\partial E_l^{\ast \prime}}{\partial E_k} \! = \! \frac{1}{2a} \frac{1}{2\sqrt{b^2 - 4 a c} } \Big( \text{-} 4 a \big( \text{-} 2 G_{k,k} E_k - G_{k,j} E_j  + \frac{\partial P^{loss}_{(l,k)} }{\partial E_k } \big) \Big) \nonumber \\
    & \frac{\partial E_l^{\ast \prime}}{\partial E_j} \! = \! \frac{1}{2a} \frac{1}{2\sqrt{b^2 - 4 a c} } \Big( \text{-} 4 a \big( \text{-} G_{k,j} E_k + \frac{\partial P^{loss}_{(l,k)} }{\partial E_j }\big) \Big) 
     \label{eq:VVextra_2} 
\end{flalign}
\normalsize
}
